# Supplementary material for: From Jam Session to Recital: Synchronous Communication and Collaboration Around Data in Organizations
Source: arXiv:2107.09042 source file (2021-07-19)
Supplement: Supplementary file 1 [file Supplemental.pdf]

# From Jam Session to Recital: Synchronous Communication and Collaboration Around Data in Organizations

Matthew Brehmer & Robert Kosara, Tableau Research
{mbrehmer,rkosara}@tableau.com

Supplemental Material for the paper accepted to IEEE VIS 2021; to appear in IEEE Transactions on Visualization & Computer Graphics.

## Interview Recruitment Screener Questions

1. Which data visualization tools have you used in the past three months? (select all that apply)
    - Power BI
    - Domo
    - Tableau
    - Excel
    - AnalyzR (fake – **reject**)
    - Qlik Sense
    - Zoho
    - I have not used any of these tools (**reject**)
2. Which of the following describes how you use data visualization tools? (select all that apply)
    - I present visualizations or dashboards in meetings (**accept**)
    - I create visualizations or dashboards and share them with others to use in presentations (**accept**)
    - I record video presentations featuring visualizations or dashboards for others to watch later (**accept**)
    - I use visualizations or dashboards that others have created (**accept only if one of the above options is selected**)
    - I create visualizations or dashboards to ask and answer questions (**accept only if one of the above options is selected**)
    - I manage or prepare data for analysis (**reject**)
    - I am a tool administrator (**reject**)
    - I provide IT infrastructure support (**reject**)
    - I do not use or support data visualization tools (**reject**)

3. How frequently have you used data visualization tools in the past three months? (select one)
    - Daily (**accept**)
    - Weekly (**accept**)
    - Monthly (**accept**)
    - Less than once a month (**reject**)
    - Never (**reject**)
4. How do you use data visualization in your job? (open-ended response)
    - …
5. On which devices do you use data visualization tools? (select all that apply)
    - Desktop
    - Laptop
    - Tablet
    - Smartphone
    - Projected display / large display
6. Which presentation tools have you used within the past 3 months? (select all that apply)
    - PowerPoint
    - Keynote
    - Google Slides
    - Quip Slides
    - Prezi
    - Other presentation tool (specify)
    - I do not use presentation tools (**reject**)

# Retrospective Interview Questions

## Intro (5 min)

We want to learn more about how you use data and data visualization when you present to others, such as in meetings, and for communication in general.

Do you have any questions for us before we get started?

## Getting to Know (40 mins)

You indicated in the screener survey that you prepare / deliver presentation materials incorporating visualization / dashboards.

1. Can you describe/show a specific example (or two) where you presented data or visuals to others?
2. What **purpose**(s) do your presentations serve?
    a. Retrospective reporting
    b. Planning
    c. Persuading / pitching / bidding for contracts / etc.

   d. Onboarding / training / orienting employees to data sources / BI tools / BI assets
   e. Other
3. Who is the **audience** of these presentations?
   a. Internal to organization: immediate colleagues / superiors / direct reports / other departments / new hires
   b. External to organization: clients / customers / general public
4. How **often** do you create presentations?
5. Do you create **new** presentations each time or do you **re-use** / **update** existing ones?
6. What **tools** do you use for preparing and delivering presentations?
   - "Slideware"
   - Tableau
   - Power BI
   - Other BI tools
   - Excel
   - Design tools
   - Other
7. How do you **incorporate data (visualization)** into presentation materials?
   a. Do you incorporate visualization / dashboards **created by others**? Who?
   b. Do you need to **reformat** visualization content for presentation? How?
8. Do you ever **record** presentation videos for asynchronous consumption? Or are all your presentations delivered live?
   a. If both, what is different about these processes? What parts of this process are difficult / tedious?
   b. If recorded, do you include **voiceover narration**? A camera feed of you?
   c. Do you create data videos / data GIFs?
   d. How / where does your audience watch these recordings?
   e. Do you ever use video editing software?
   f. How often do you watch recorded presentations featuring visualization? What do you like / not like about these?
9. When delivering / recording presentations, do you have a **second display**?
   a. What is on this second display? Notes / secondary application / presenter view?
   b. If they don't have a second screen, would they use one if they did? How?
   c. In live-colocated presentations, do you ever use pointers, clickers, or mobile presentation apps for highlighting or advancing slides?

10. Do you **distribute presentation materials** or recordings before or after a live presentation?
    a. If yes, are there appendices with more data? Pointers to dashboards?
11. Do you want the data to be **live** and **up-to-date** during the presentation? Or are static snapshots of the data sufficient?
    a. Do you want to control or filter the data during a presentation?
    b. Do you want to be able to answer questions about the data during the presentation or meeting?
12. How do you use **builds / transitions / animations / reveals** in your presentations? If not, why not?
    a. How would you want to incorporate such aspects in your presentations beyond what is currently possible / easily achievable?
    b. What does the term “progressive reveal” or “incremental reveal” mean to you in the context of visualization?
13. How do you **annotate or highlight** visualizations when using them in presentations?
    a. How would you want to annotate or highlight them beyond what is currently possible / easily achievable?
14. What kinds of things are difficult to do today?
15. What would you want to be able to do?
16. What would an ideal presentation look like?

## Conclusion (5 min)

- After what you’ve seen and what we’ve talked about, if you had a **magic wand** and could make anything happen, what would your ideal scenario of presenting data look like?
- Do you have any additional questions for us?
- Thank you for being generous with your time. We really appreciate all of the things you have told us about your presentation process and your feedback on our concepts.
- Do you have colleagues / friends that could provide alternative perspectives that you could refer to us?
- Can we email you with follow-up questions?

# Design Probe Interview Questions

We want to learn more about how people use data and visualization when they present to others, like in meetings, and for communication in general.

We are going to show you a few sketches of ideas in a few moments, where the goal is to think broadly about these kinds of uses, not the specific mock-ups you will see. We're looking for inspiration and to explore ideas, and we want to think beyond what you are able to do right now. It's really about high-level feedback, we don't want to get hung up on little things like details of the user interface, since those will undoubtedly change.

We are looking for your honest feedback, though, so please don't hesitate if there are things that you don't think are useful, or that you think would be confusing or otherwise not helpful for your work.

## Getting to Know (15 mins)

First, a few questions about you and your work

- What data do you use for presentation?
- Do you create presentation materials for others?
- Walk us through how you build a presentation, get the data, build the presentation, present, etc. – what are the pain points
  - What tools do you use?
    - Data access and analysis
    - Presentation tools/“slideware”
    - Other (white boards, etc.)
  - Do you use features like animations, reveals, builds, etc.?
  - Do you work with others?

## Design Probes (3 x 10 mins)

*[**Author's note**: each of the three design probes are profiled in the supplemental video, however, as stated in the paper: “We consolidated these videos into a single presentation accompanied by a scripted explanation; we provide a recording as supplemental material.” Video clips in the supplemental video are edited and sped up for the sake of brevity, while our interviewees saw unedited versions at 1x playback speed; we provided an accompanying scripted explanation live, which allowed for interruptions and pauses to ensure that the interviewee understood the concept and had an opportunity to ask clarifying questions. We did not have prepared questions for these design probes beyond those stated below. Instead, the conversation about these design probes was left open-ended.]*

Now we want to show you three concepts that we've been working on

- The Progressive Reveal of Charts & Dashboards [see supplemental video: 0:05 – 1:28]
    - Our first concept pertains to progressive reveal, Our first concept pertains to progressive reveal.
    - What does the term “progressive reveal” or “incremental reveal” mean to you in the context of dashboards / visualization?
    - Imagine you have a worksheet of line and bar charts, where you have several data categories represented by mark color, in this example the three colors correspond to three companies. This video shows a way of revealing the data one category at a time, without affecting other parts of the worksheet, such as the legend or the ranges along the axes.
    - Or consider a line chart in which you control the rate at which the lines get revealed. While it’s already possible in Tableau to reveal everything at once or one year after another, let’s say you want to reveal the first few time steps, 2000, 2001, and 2002 then you want to jump ahead to the last couple time steps in this dataset: 2011 and 2012. So that when you begin the reveal, you show the first three years, and then you jump ahead to the last 2 years. Or you could jump back and forth between these pre-specified reveal steps.
    - What if you want to progressively reveal marks along a continuous measure, such as the population of countries, which in this example corresponds to the size of marks in this scatterplot. Rather than reveal all countries at once, let’s first reveal the countries with a population of 100 million or more, and then let’s reveal all the others. Alternatively, let’s change the reveal order to reveal the countries with more than 100 million people but less than a billion, and then let’s reveal the countries with a billion or more.
    - So far, we’ve only talked about the progressive reveal of marks in a visualization. Here we move up a level to reveal parts of a worksheet, such as first revealing the gridlines and zero lines of a chart, then the axis labels and headers, then the marks, in this case revealing marks belonging to one set before all of the remaining marks, and finally we reveal the annotation layer.
    - While that reveal order might be a decent default, let’s say you want to customize it, such that one group of marks appears simultaneously with an annotation, so you’d need to create a new reveal group, add the desired marks and annotation to that group, and then move this group into its appropriate place in the reveal order.
    - Now when we step through our new reveal order, one group of marks and its associated annotation appear before the remaining marks and the other annotation.
    - Before we introduce the next concept, I’ll pause and ask you about your first impressions in response to this concept of progressively revealing parts of a visualization or worksheet.

- Second-Screen Controls for Presenting Data [see supplemental video: 1:29 – 2:03]

- If you are connected to an external display in a live meeting in which you are presenting visualization, what would you want on your personal display? Mirror the displays? or something else?
- You might be familiar with the presenter view in presentation programs like PowerPoint and Keynote. This is the same idea, at its heart, but it's more geared towards data presentation. Here you see a simple presenter view where you would see on your screen what is currently being shown on the presentation screen in the large image on the left, as well as a small preview of the next step over on the right, plus also your speaker notes.
- The idea being that you could use this to step through reveals you had set up, like the way I just showed you, and see what the next step would look like. And in this case, we're starting the presentation by showing the top of a dashboard first before we dive into more details.
- So here we have the next step, which is now showing additional product-level detail about shipping, which might be relevant to understand the data at the top. But we want to go a bit further and actually do some interaction with the dashboard during the presentation. To do that without having to squint at the screen or have the audience see our mouse pointer move around, we've torn off the filters from the dashboard.
- So now here you can see the filter panel on the right, which is only visible to the presenter, and the dashboard without its filters that is being shown to the audience. The idea is that I can now use this as a controller while presenting. Perhaps I want to compare Q4 to Q4, I can just change the filter.
- And the dashboard that the audience sees responds, of course. They don't need to see how I did that, as long as I tell them what I'm doing of course.
- What are your thoughts on this part?

- Coordinating Recorded Video with Interactive Visualization [see video 2:04 – 3:19]
  - How often do you record presentations involving data so that your audience can consume later?
  - How often do you watch recorded presentations that involve data?
  - What are some of the issues or drawbacks that you encounter with respect to producing or consuming recorded presentations that involve data?
  - The last concept that we'd invite your feedback on addresses a scenario that has perhaps become more common with everyone working from home and balancing a different work-life schedule, and that is consuming presentations asynchronously, but still being able to interact with the content.
  - Our idea here is an interactive coordination between a presenter's video and dashboard content. Here you see a video player embedded within a dashboard, which in this case happens to be about books and authors. The video is synchronized with the dashboard and the video timeline is augmented with interactive waypoints that correspond with changes in the dashboard, and each waypoint has a portion of the video's transcript displayed beside it, either a verbatim transcript of the presenter's monologue or a summary caption for the

corresponding state of the dashboard. Unlike a recorded video, the audience can interact with the content during the video presentation, or they can navigate to states of a dashboard that are associated with a waypoint in the video presentation. And since the presenter video is prominent and in a fixed location within the dashboard, they can still use gestures and spatial references like "the visualization to my left" or "the visualization below my video". This is unlike most remote presentations in which the presenter's video feed is relegated to a tiny floating thumbnail that is ignored or buried behind other windows, and it's also unlike other recorded presentations in that you can interact with the content: it's still a live interactive dashboard. The overall aim with this concept is to bring some human connection between presenter and audience that we're used to live in-person presentations in recorded presentations.

- Here is a recap of how the video player coordinated with the dashboard throughout that demo. Starting with an initial dashboard state, new content got added, some content got spotlighted, some content was replaced with other content, filter and parameter settings were updated, and annotation in the form of text, images, and reference lines were added and removed at different points throughout the video.
- This demo illustrates what an authoring interface could look like, or how a presenter would prepare a presentation that coordinates video and their dashboard. In which a presenter loads a video and configures a dashboard to record snapshots of the dashboard at different points in the video, and for each waypoint they could also control the visibility of various parts of the dashboard.
- Interactive coordination between video and visualization content could also extend beyond dashboards: It might also be a new form of content to share on online platforms like Tableau Public, which could be embedded elsewhere on the web.
- These types of interactive recorded presentations might also be consumable via a mobile app.
- This coordination between video and an interactive dashboard could be useful not only for delivering presentations, but also for onboarding people to an unfamiliar dashboard or workbook.
- What are your first impressions in response to this concept of coordinating video with an interactive dashboard?

## Card Sorting (5 mins)

Pick top three, order those in increasing order of desirability. Think about yourself, not what you think others might want.

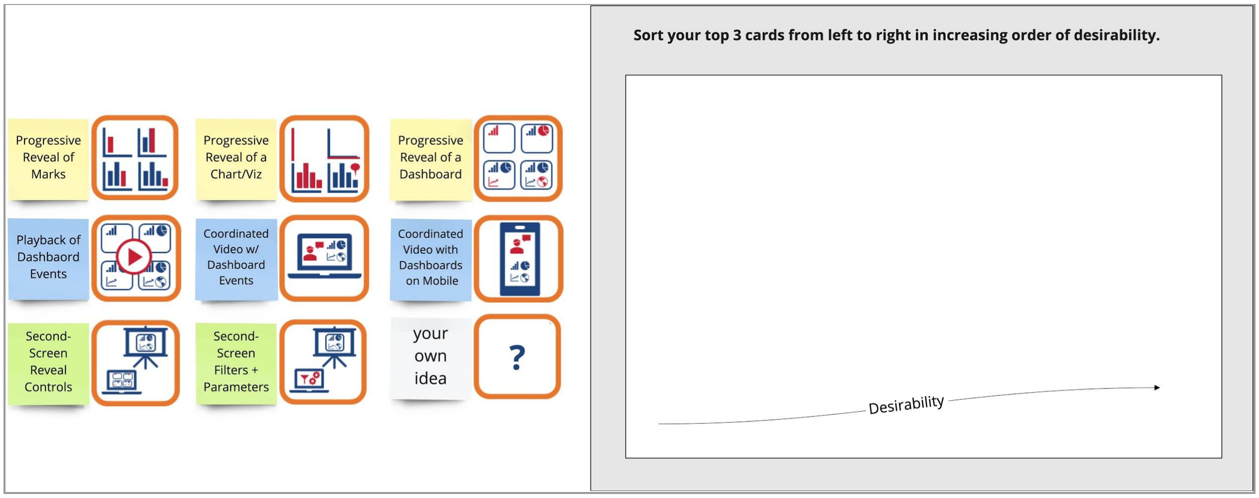


- Why did you pick these three cards? Why did you order them in this way?

[**Authors' note**: *We determined the results from the card sorting exercise to be inconclusive; we therefore decided to omit these results from the paper, opting instead to focus on reporting interviewees' responses to our open-ended questions*. ]

## Conclusion (5 mins)

After what you've seen and what we've talked about, if you had a magic wand and could make anything happen, what would your ideal scenario of presenting data look like?
